# Supplementary material for: Iterative Graph Neural Network Enhancement via Frequent Subgraph Mining of Explanations
Source: arXiv:2403.07849 source file (2024-03-12)
Supplement: Supplementary file 2 [file tab-02.tex]

\begin{tabular}{lr}
  \toprule
  & F1-Score \\
  \midrule
  Label Encoded (LE) & 100.00 \\
  Adversarial (A)    &  78.08 \\
  Random (R)         &  86.07	\\
  EEGL Round-0       &  60.55 \\
  EEGL Round-1       & 100.00 \\ \hline
\end{tabular}
